# Supplementary material for: Exploring Conditional Text Generation for Aspect-Based Sentiment Analysis
Source: arXiv:2110.02334 source file (2021-10-07)
Supplement: Supplementary file 1 [file 7-Appendix.tex]

% 
% T5-ASD table results
% 
\begin{table}[!htb]
    \centering
    \resizebox{\linewidth}{!}{%
        \begin{tabular}{|l|rr|rr|}
            \hline
            \multicolumn{1}{|c|}{\multirow{2}{*}{\begin{tabular}[c]{@{}c@{}}sentence/\\ phrase\end{tabular}}} &
            \multicolumn{2}{c|}{AD}                                & \multicolumn{2}{c|}{ASD}                               \\
            \multicolumn{1}{|c|}{}                                 & \multicolumn{1}{c}{SE-15} & \multicolumn{1}{c|}{SE-16} & \multicolumn{1}{c}{SE-15} & \multicolumn{1}{c|}{SE-16} \\ \hline
            sen-1 & 78.98          & 84.95          & 70.87          & 78.68          \\
            sen-2 & 78.79          & \textbf{85.24} & 70.47          & \textbf{79.00} \\
            sen-3 & \textbf{79.11} & 85.20          & \textbf{71.00} & 78.56          \\ \hline
            phr-1 & 78.24          & 83.94          & 70.94          & 77.92          \\
            phr-2 & \textbf{79.45} & \textbf{84.05} & \textbf{71.65} & \textbf{78.09} \\
            phr-3 & 78.42          & 84.00          & 70.97          & 77.95          \\ \hline
        \end{tabular}%
    }
    \caption{Results for T5-ASD on SE-15 and SE-16}
    \label{tab: T5-ASD}
\end{table}

% 
% T5-TSD table results
% 
\begin{table}[!htb]
    \centering
    \resizebox{\linewidth}{!}{%
        \begin{tabular}{|l|rr|rrrr|}
            \hline
            \multicolumn{1}{|c|}{\multirow{2}{*}{\begin{tabular}[c]{@{}c@{}}sentence/\\ phrase\end{tabular}}} &
              \multicolumn{2}{c|}{TD} &
              \multicolumn{4}{c|}{TSD} \\
            \multicolumn{1}{|c|}{} &
              \multicolumn{1}{c}{SE-15} &
              \multicolumn{1}{c|}{SE-16} &
              \multicolumn{2}{c}{SE-15} &
              \multicolumn{2}{c|}{SE-16} \\ \hline
            sen-1 & 79.28          & 81.88          & 70.37          & 70.43          & 76.66          & 75.74          \\
            sen-2 & 79.53          & 81.54          & \textbf{71.04} & \textbf{70.82} & \textbf{76.75} & \textbf{76.03} \\
            sen-3 & \textbf{79.60} & \textbf{82.02} & 70.68          & 70.69          & 76.53          & 75.64          \\ \hline
            phr-1 & 78.69          & \textbf{83.32} & 69.97          & 70.58          & \textbf{78.03} & \textbf{77.40} \\
            phr-2 & 79.12          & 82.75          & 70.52          & 71.00          & 77.85          & 77.32          \\
            phr-3 & \textbf{79.38} & 82.70          & \textbf{70.95} & \textbf{71.46} & 77.39          & 77.00          \\ \hline
        \end{tabular}%
    }
    \caption{Results for T5-TSD on SE-15 and SE-16}
    \label{tab: T5-TSD}
\end{table}

% 
% T5-TAD
% 
\begin{table}[!htb]
    \centering
    \resizebox{\linewidth}{!}{%
        \begin{tabular}{|l|rr|rr|rr|}
            \hline
            \multicolumn{1}{|c|}{\multirow{2}{*}{\begin{tabular}[c]{@{}c@{}}sentence/\\ phrase\end{tabular}}} &
              \multicolumn{2}{c|}{AD} &
              \multicolumn{2}{c|}{TD} &
              \multicolumn{2}{c|}{TAD} \\
            \multicolumn{1}{|c|}{} &
              \multicolumn{1}{c}{SE-15} &
              \multicolumn{1}{c|}{SE-16} &
              \multicolumn{1}{c}{SE-15} &
              \multicolumn{1}{c|}{SE-16} &
              \multicolumn{1}{c}{SE-15} &
              \multicolumn{1}{c|}{SE-16} \\ \hline
            sen-1 & 77.41          & \textbf{84.62} & \textbf{80.65} & 83.56          & 66.46          & \textbf{73.02} \\
            sen-2 & 77.84          & 83.66          & 79.84          & \textbf{84.30} & 66.32          & 72.70          \\
            sen-3 & \textbf{77.98} & 83.64          & 80.14          & 83.79          & \textbf{66.48} & 72.56          \\ \hline
            phr-1 & \textbf{77.43} & 82.59          & \textbf{80.73} & 82.41          & 67.39          & 73.50          \\
            phr-2 & 77.10          & \textbf{82.97} & 80.70          & \textbf{82.76} & \textbf{67.53} & \textbf{74.07} \\
            phr-3 & 76.77          & 82.78          & 80.71          & 82.55          & 67.16          & 73.99          \\ \hline
        \end{tabular}%
    }
    \caption{Results for T5-TAD on SE-15 and SE-16 datasets}
    \label{tab: T5-TAD}
\end{table}

% 
% T5-TASD
% 
% Please add the following required packages to your document preamble:
% \usepackage{multirow}
% \usepackage{graphicx}
\begin{table*}[]
    \centering
    \resizebox{\textwidth}{!}{%
        \begin{tabular}{|l|rr|rr|rr|rr|rrrr|rrrr|}
            \hline
            \multicolumn{1}{|c|}{\multirow{2}{*}{\begin{tabular}[c]{@{}c@{}}sentence/\\ phrase\end{tabular}}} &
              \multicolumn{2}{c|}{AD} &
              \multicolumn{2}{c|}{TD} &
              \multicolumn{2}{c|}{TAD} &
              \multicolumn{2}{c|}{ASD} &
              \multicolumn{4}{c|}{TSD} &
              \multicolumn{4}{c|}{TASD} \\
            \multicolumn{1}{|c|}{} &
              \multicolumn{1}{c}{SE-15} &
              \multicolumn{1}{c|}{SE-16} &
              \multicolumn{1}{c}{SE-15} &
              \multicolumn{1}{c|}{SE-16} &
              \multicolumn{1}{c}{SE-15} &
              \multicolumn{1}{c|}{SE-16} &
              \multicolumn{1}{c}{SE-15} &
              \multicolumn{1}{c|}{SE-16} &
              \multicolumn{2}{c}{SE-15} &
              \multicolumn{2}{c|}{SE-16} &
              \multicolumn{2}{c}{SE-15} &
              \multicolumn{2}{c|}{SE-16} \\ \hline
            sen-1 &
              77.98 &
              \textbf{82.97} &
              79.42 &
              83.53 &
              67.14 &
              72.93 &
              70.29 &
              \textbf{76.05} &
              71.17 &
              70.60 &
              \textbf{76.50} &
              \textbf{77.20} &
              61.03 &
              \textbf{55.70} &
              67.30 &
              57.70 \\
            sen-2 &
              \textbf{78.58} &
              82.77 &
              79.41 &
              83.02 &
              \textbf{67.72} &
              72.91 &
              \textbf{70.55} &
              75.98 &
              \textbf{71.57} &
              70.75 &
              75.77 &
              76.55 &
              61.15 &
              55.57 &
              67.40 &
              55.79 \\
            sen-3 &
              78.00 &
              82.77 &
              79.67 &
              \textbf{83.54} &
              67.51 &
              \textbf{73.03} &
              70.25 &
              75.69 &
              71.50 &
              \textbf{70.82} &
              76.28 &
              76.89 &
              \textbf{61.15} &
              55.34 &
              \textbf{67.48} &
              \textbf{58.14} \\
            combiation &
              77.85 &
              82.50 &
              \textbf{79.98} &
              83.40 &
              66.55 &
              72.19 &
              69.72 &
              75.35 &
              71.28 &
              70.66 &
              76.38 &
              76.74 &
              60.40 &
              54.55 &
              67.03 &
              57.78 \\ \hline
            phr-1 &
              76.97 &
              83.04 &
              80.30 &
              82.91 &
              66.57 &
              74.30 &
              70.03 &
              76.64 &
              71.60 &
              \textbf{72.16} &
              76.53 &
              77.76 &
              61.25 &
              52.60 &
              69.26 &
              55.50 \\
            phr-2 &
              \textbf{77.31} &
              \textbf{83.10} &
              80.48 &
              82.98 &
              \textbf{67.19} &
              74.23 &
              \textbf{70.13} &
              \textbf{77.17} &
              \textbf{71.60} &
              71.98 &
              \textbf{77.07} &
              78.19 &
              \textbf{61.42} &
              52.02 &
              69.60 &
              \textbf{55.77} \\
            phr-3 &
              76.98 &
              82.95 &
              80.09 &
              83.33 &
              66.54 &
              \textbf{74.65} &
              69.63 &
              76.80 &
              70.77 &
              71.30 &
              76.93 &
              \textbf{78.22} &
              60.60 &
              52.77 &
              \textbf{69.85} &
              55.32 \\
            combiation &
              77.25 &
              82.48 &
              \textbf{80.69} &
              \textbf{83.51} &
              66.08 &
              73.34 &
              69.88 &
              76.15 &
              71.29 &
              71.72 &
              76.78 &
              78.10 &
              60.92 &
              \textbf{53.06} &
              69.01 &
              54.62 \\ \hline
        \end{tabular}%
    }
    \caption{Results for T5-TASD on SE-15 and SE-16 datasets}
    \label{tab: T5-TASD}
\end{table*}
